# Supplementary material for: Computing Medial Axis Transform with Feature Preservation via Restricted Power Diagram
Source: arXiv:2210.13676 source file (2022-10-25)
Supplement: Supplementary file 1 [file 8_appendix.tex]

\section{Appendix}

\subsection{External Edge Feature Preservation}
\label{sec:app_sharpline}

\begin{figure}[h]
    \centering
	\includegraphics[width=\linewidth]{figs/appendix/ext_deletion.jpeg}
	\caption{(a) Illustration of RPD of three medial spheres $\msphere_a =(\mcenter_a,0)$, $\msphere_b =(\mcenter_b,0)$, and $\msphere_i =(\mcenter_i, r_i)$, where $\msphere_a$ and $\msphere_b$ are two neighboring zero-radius medial spheres, and $\msphere_i$ is a non-feature medial sphere neighboring to $\msphere_a$ and $\msphere_b$ with radius $r_i$. Plane $\Pi[\msphere_a,\msphere_b]$ is the bisecting plane defined by $\msphere_a$ and $\msphere_b$, and intersects the feature edge at point $\mathbf{p}$. Plane $\Pi[\msphere_a,\msphere_i]$ is the bisecting plane defined by spheres $\msphere_a$ and $\msphere_i$ using power distance, and intersects the feature edge at point $\mathbf{q}$. (b)-(d) show three different relations between $\mathbf{p}$, $\mathbf{q}$, and $\msphere_a$. (b): Points $\mathbf{p}$ and $\mathbf{q}$ overlap. (c): Point $\mathbf{q}$ is closer to $\mcenter_a$ than point $\mathbf{p}$ is. (d): Point $\mathbf{p}$ is closer to $\mcenter_a$ than point $\mathbf{q}$ is.
    }
	\label{fig:app_ext_deletion}
\end{figure}

One possible fix for the problem shown in Fig.~\ref{fig:extf_add_se} of the paper is to insert new feature spheres when the non-feature medial sphere whose RPC intrudes into the connection borders between two RPCs of neighboring zero-radius spheres on a sharp edge. 

Suppose we have a non-feature medial sphere $\msphere_i =(\mcenter_i,r_i)$, and two neighboring zero-radius feature spheres represented as $\msphere_a =(\mcenter_a,0)$, $\msphere_b=(\mcenter_b,0)$ respectively, as shown in Fig.~\ref{fig:app_ext_deletion}. Note that we place zero-radius spheres $\msphere_a$ and $\msphere_b$ on the external feature edge, so the two neighboring medial spheres $\msphere_a$ and $\msphere_b$ are supposed to be connected in our final medial mesh without the interference of any non-feature medial sphere $\msphere_i$. That means, the RPC of $\msphere_i$, represented as $\rpc_{i}$, should not intersect the feature edge $\mathbf{\mcenter_a \mcenter_b}$ in between $\msphere_a$ and $\msphere_b$.

The boundary of the power cell of $\msphere_a$ is defined by its bounding planes $\{\Pi[\msphere_a,\msphere_i] | i=1... m\}$, where any point on the plane $\Pi[\msphere_a,\msphere_i]$ is of equal power distance to these two medial spheres $\msphere_a$ and $\msphere_i$. Note that $\{\msphere_i|i=1...m\}$ are the neighboring medial spheres of $\msphere_a$. Apparently $\Pi[\msphere_a,\msphere_b]$ is a bisector between two centers $\mcenter_a$ and $\mcenter_b$ since they have the same zero radius. Suppose plane $\Pi[\msphere_a,\msphere_b]$ intersects the feature edge ${\mathbf{\mcenter_a \mcenter_b}}$ on point $\mathbf{p}=\frac{1}{2}(\mcenter_a+\mcenter_b)$. For any non-feature medial sphere $\msphere_i$ that is in the vicinity of $\msphere_a$, the plane $\Pi[\msphere_a,\msphere_i]$ intersects the feature edge ${\mathbf{\mcenter_a \mcenter_b}}$ on point $\mathbf{q}$. 

We can tell whether the connection between $\msphere_a$ and $\msphere_b$ is invaded by $\msphere_i$ based on the relationship between $\mathbf{p}$, $\mathbf{q}$, and the center $\mcenter_a$ on the feature edge: if point $\mathbf{q}$ is closer to $\mcenter_a$ than point $\mathbf{p}$ (Fig.~\ref{fig:app_ext_deletion} (c)), then $\mathbf{p}$ cannot be preserved in the final RPD, so the connection between $\msphere_a$ and $\msphere_b$ is invaded by $\msphere_i$. To avoid handling degeneracy, we also exclude the case when $\mathbf{p}=\mathbf{q}$ (Fig.~\ref{fig:app_ext_deletion} (b)). This means $d_{pow}(\mathbf{p},\msphere_a) \geq d_{pow}(\mathbf{p},\msphere_i)$, which results in the following inequation:
\begin{equation}\label{eq:line_feature_preservation}
    \mcenter_i^{\top}\mcenter_i - (\mcenter_a+\mcenter_b)^{\top}\mcenter_i + \mcenter_a^{\top}\mcenter_b \leq r_i^2.
\end{equation}
In summary, new zero-radius medial spheres should be inserted if the above Eq.~\eqref{eq:line_feature_preservation} is satisfied for non-feature sphere $\msphere_i$.

\subsection{Algorithms}
\label{sec:app_algo}
In this section we provide the detailed algorithms of (1) seam tracing as discussed in Sec.~\ref{sec:init_mm}, and (2) geometry-guided thinning as discussed in Sec.~\ref{sec:refine}.

\newpage

\begin{algorithm}
\caption{Seam Tracing}\label{alg:seam_tracing}
\KwData{$\mmesh$ = \{\{$\msphere_i$\}, \{$e_{ij}$\}, \{$f_{ijw}$\}\},  the medial mesh of shape $\model$}
\KwResult{$E$ = \{$e_{ij}$\}, the edges on internal features}
$Q \gets \varnothing$ \tcp{queue of medial spheres on seams} %\;
\For{each vertex $\msphere_i$ in $\mmesh$ of type $T_N$ with $N > 2$} {
    $Q \gets \msphere_i$
}
\While{$Q$ not empty}{
    $\msphere_i \gets Q.top()$ \\
    \If{$\msphere_i$ has 2 incident edges in E}{
        continue\;
    }
    \For{each neighbors $\msphere_j$ of $\msphere_i$}{
        \uIf{$\msphere_j$ on external feature}{
            store edge $e_{ij}$ = \{$\msphere_i$, $\msphere_j$\} in $E$
        }
        \uElseIf{all CCs of $\msphere_i$ adjacent to CCs of $\msphere_j$}{
            store edge $e_{ij}$ = \{$\msphere_i$, $\msphere_j$\} in $E$
        }
    }
}
\end{algorithm}

\begin{algorithm}
\caption{Geometry-guided Thinning}\label{alg:thinning}
% This is to hide end and get the last vertical line straight
\KwData{$\mmesh$ = \{\{$\msphere_i$\}, \{$e_{ij}$\}, \{$f_{ijw}$\}, \{$t_{ijwk}$\}\}, the medial mesh of shape $\model$, which contains tetrahedra \{$f_{ijw}$\}}
\KwData{$\sigma$, the target important factor; when reaching this, the face-edge pair \{$f_{ijw}$, $e_{ij}$\} will be not deleted}
\KwResult{$\overline{\mmesh}$ = \{\{$\msphere_i$\}, \{$e_{ij}$\}, \{$f_{ijw}$\}\}, the pruned medial mesh without any tetrahedron}
$Q \gets \varnothing$ \tcp{priority queue of $f_{ijw}$ sorted by  importance factor $\alpha_{ijw}$}%\;
\For{each face $f_{ijw}$ in non-deleted tet $t_{ijwk}$} {
    compute the importance factor $\alpha_{ijw}$\;
    $Q \gets f_{ijw}$ with $\alpha_{ijw}$
}
\tcc{Prune tet-face simple pairs}
\While{number of non-deleted $t_{ijwk} \neq 0$}{
    \For{each $f_{ijw}$ in $Q$}{
        \If{$f_{ijw}$ is not delete and $f_{ijw}$ is adjacent to only 1 tet $t_{ijwk}$}{
            prune tet-face pair \{$t_{ijwk}$, $f_{ijw}$\} \;
            break\;
        }
    }
}
\tcc{Prune face-edge simple pairs}
$n_f \gets 0$ \tcp{number of faces on tets that have been processed}
\While{$n_f \neq Q.size()$}{
    $n_f \gets 0$\\
    \For{each $f_{ijw}$ in $Q$}{
        \If{$f_{ijw}$ is deleted or $\alpha_{ijw} \geq \sigma$}{
            $n_f++$\;
            continue\;
        }
        \For{each $e_{ij}$ in $f_{ijw}$}{
            \If{$e_{ij}$ is adjacent to only 1 face $f_{ijw}$ and not on external features}{
                prune face-edge pair \{$f_{ijw}$, $e_{ij}$\} \;
                break\;
            }
        }
        \If{$f_{ijw}$ is deleted}{
            break\;
        }
        $n_f++$\;
    }
}
\end{algorithm}
